# Supplementary material for: A Neural Conversational Model
Source: arXiv:1506.05869 source file (2015-07-22)
Supplement: Supplementary file 1 [file appendix.tex]

\section{A full conversation with the model trained on OpenSubtitles}
